# Supplementary material for: Challenges and Advancements in Modeling Shock Fronts with Physics-Informed Neural Networks: A Review and Benchmarking Study
Source: arXiv:2503.17379 source file (2025-03-14)
Supplement: Supplementary file 1 [file t_SI.tex]

\begin{table}[ht]

\caption{A summary of the studies worked on applying PINNs for solving spontaneous imbibition (SI) problem.}
\begin{center}
    \label{tab:SI}
    \begin{tabular}[t]{ll}
    \hline
    Reference & Summary  \\ \hline

    Deng and Pan \cite{Deng2021ApplicationImbibition} & ...  \\ \hline
    Abbasi and Andersen \cite{Abbasi2023SimulationNetworks} & \makecell{... }  \\ \hline    
    ...  & \makecell{2D evaluations }  \\ \hline    
        
    \end{tabular}
\end{center}
\end{table}
